# Supplementary material for: Causal Retrieval with Semantic Consideration
Source: arXiv:2504.04700 source file (2026-03-09)
Supplement: Supplementary file 1 [file appendix_causal.tex]

\begin{table*}[hbt!]
\setlength{\tabcolsep}{1pt}

\scriptsize{
\resizebox{\textwidth}{!}{
\begin{tabular}{l|ccc|ccc|ccc|ccc|ccc|ccc}
    \toprule
    \multirow{3}{*}{\centering\textbf{Model}} 
    & \multicolumn{9}{c}{\textbf{Task 1. Cause to Effect}} 
    & \multicolumn{9}{c}{\textbf{Task 2. Effect to Cause}} \\
    \cmidrule(lr){2-10} \cmidrule(lr){11-19}
    & \multicolumn{3}{c}{\textbf{e-CARE}} 
    & \multicolumn{3}{c}{\textbf{e-CARE + $\text{wiki}_{XL}$}} 
    & \multicolumn{3}{c}{\textbf{e-CARE + $\text{RedPajama}_{XL}$}}  
    & \multicolumn{3}{c}{\textbf{e-CARE}} 
    & \multicolumn{3}{c}{\textbf{e-CARE + $\text{wiki}_{XL}$}} 
    & \multicolumn{3}{c}{\textbf{e-CARE + $\text{RedPajama}_{XL}$}}  \\
    \cmidrule(lr){2-4} \cmidrule(lr){5-7} \cmidrule(lr){8-10} 
    \cmidrule(lr){11-13} \cmidrule(lr){14-16} \cmidrule(lr){17-19}  
    & Hit@1 & Hit@10 & MRR@10 & Hit@1 & Hit@10 & MRR@10 & Hit@1 & Hit@10 & MRR@10 
    & Hit@1 & Hit@10 & MRR@10 & Hit@1 & Hit@10 & MRR@10 & Hit@1 & Hit@10 & MRR@10  \\
    \midrule
    
    \ours-DPR-causal
     & 38.4 & 68.7 & 47.9
     & 18.0 & 32.5 & 22.2
     & 15.4 & 28.7 & 19.3
     & 39.0 & 67.2 & 47.6
     & 20.6 & 35.6 & 25.2
     & 18.0 & 32.6 & 22.2
    \\
    
    \ours-GTR-causal
    & 43.2 & 69.7 & 51.2
    & 27.1 & 43.0 & 31.5
    & 24.6 & 40.3 & 29.2
    & 42.7 & 68.8 & 50.8
    & 27.5 & 42.6 & 32.3
    & 25.6 & 40.7 & 30.1\\
    
    \ours-BGE M3-causal
    & 44.9 & 71.3 & 52.7
    & 29.6 & 44.9 & 33.9
    & 26.6 & 41.9 & 31.0
    & 44.4 & 71.9 & 52.7
    & 31.3 & 46.2 & 36.0
    & 27.7 & 42.6 & 32.4\\

    % \hline

    % ColBERT
    % & 37.4 & 67.5 & 46.8
    % & 17.4 & 33.0 & 21.8
    % & 14.5 & 27.9 & 18.4
    % & 37.8 & 66.6 & 46.7
    % & 18.4 & 33.4 & 23.1
    % & 14.9 & 29.0 & 19.2 \\

    % \ours-ColBERT
    % & 32.2 & 58.6 & 40.1
    % & 17.1 & 28.9 & 20.7
    %  & 14.9 & 24.5 & 17.7
    % & 36.4 & 62.0 & 44.3
    % & 21.0 & 34.9 & 25.3
    %  & 18.4 & 30.1 & 21.9 \\
    
    \bottomrule
\end{tabular}}
}
\caption{Accuracy comparison on e-CARE}
%Task 1 is to retrieve an effect sentence given a cause query, and Task 2 is to retrieve a cause sentence given an effect. }
\label{appendix_causalloss}
\end{table*}
